# Supplementary material for: Significant-loophole-free test of Bell's theorem with entangled photons
Source: arXiv:1511.03190 ancillary file (2015-12-20)
Supplement: Supplementary file 1 [file supplemental_material_Vienna_20151220.pdf]

# Supplemental Material: Significant-Loophole-Free Test of Bell's Theorem with Entangled Photons

Marissa Giustina,<sup>1,2,\*</sup> Marijn A. M. Versteegh,<sup>1,2</sup> Sören Wengerowsky,<sup>1,2</sup> Johannes Handsteiner,<sup>1,2</sup> Armin Hochrainer,<sup>1,2</sup> Kevin Phelan,<sup>1</sup> Fabian Steinlechner,<sup>1</sup> Johannes Kofler,<sup>3</sup> Jan-Åke Larsson,<sup>4</sup> Carlos Abellán,<sup>5</sup> Waldimar Amaya,<sup>5</sup> Valerio Pruneri,<sup>5,6</sup> Morgan W. Mitchell,<sup>5,6</sup> Jörn Beyer,<sup>7</sup> Thomas Gerrits,<sup>8</sup> Adriana E. Lita,<sup>8</sup> Lynden K. Shalm,<sup>8</sup> Sae Woo Nam,<sup>8</sup> Thomas Scheidl,<sup>1,2</sup> Rupert Ursin,<sup>1</sup> Bernhard Wittmann,<sup>1,2</sup> and Anton Zeilinger<sup>1,2,†</sup>

<sup>1</sup>*Institute for Quantum Optics and Quantum Information (IQOQI),  
Austrian Academy of Sciences, Boltzmannngasse 3, Vienna 1090, Austria.*

<sup>2</sup>*Quantum Optics, Quantum Nanophysics, and Quantum Information,  
Faculty of Physics, University of Vienna, Boltzmannngasse 5, Vienna 1090, Austria*

<sup>3</sup>*Max-Planck-Institute of Quantum Optics, Hans-Kopfermann-Straße 1, 85748 Garching, Germany*

<sup>4</sup>*Institutionen för Systemteknik, Linköpings Universitet, 581 83 Linköping, Sweden*

<sup>5</sup>*ICFO – Institut de Ciències Fòniques, The Barcelona Institute of Science and Technology, 08860 Castelldefels, Barcelona, Spain*

<sup>6</sup>*ICREA – Institució Catalana de Recerca i Estudis Avançats, 08015 Barcelona, Spain*

<sup>7</sup>*Physikalisch-Technische Bundesanstalt, Abbestraße 1, 10587 Berlin, Germany*

<sup>8</sup>*National Institute of Standards and Technology (NIST), 325 Broadway, Boulder, Colorado 80305, USA*

(Dated: December 20, 2015)

## I. ENTANGLED PHOTON SOURCE AND FIBER CHANNELS

The source of entangled photons [Fig. 1] uses a periodically poled potassium titanyl phosphate (ppKTP) crystal in a Sagnac configuration [1], which has proven suitable for high heralding efficiencies [2]. The pump laser (Omicron TA Deepstar) is pulsed with a repetition rate of 1 MHz and a pulse length of 12 ns. After traversing a single-mode fiber for spatial filtering, the pump beam is collimated and focused with two lenses to a Gaussian beam waist radius of 170  $\mu\text{m}$  in the ppKTP crystal. Here, the 405 nm pump photons produce photon pairs at 810 nm via type II spontaneous parametric down-conversion (SPDC). The focusing parameters are optimized for a high heralding efficiency [3, 4]. Every second, about 3 500 pairs are created in the crystal in our collection mode (waist radius 65  $\mu\text{m}$ ), which overlaps with the pump beam inside the crystal. The near-optimal alignment of the entangled photon source is reflected in total heralding efficiencies of approximately 78.6% and 76.2% for Alice and Bob respectively. Correcting for the estimated losses in the polarization module and the long fibers, which amount to approximately 10%, we can infer single-mode heralding efficiencies of approximately 87% and 85% when measured directly at the source. (Note that these values are not corrected for the detection efficiency, which is assumed to be near-unity [5].) These are among the highest values reported to date.

Both SPDC photons are collected by two-lens systems consisting of a lens for collimation and a lens to focus into 32.0 m  $\pm$  0.5 m long single mode fibers connecting the source with the measurement stations Alice and Bob on each side. Stress-induced birefringence in the fibers is tuned in manual polarization controllers (POLC) to ensure that the horizontal-vertical (HV) basis of the polarizing beam splitter cube (PBS) in the source is identical to the HV basis of the polarizers in

the measurement stations. For the fibers, no active temperature stabilization is used, but the HV basis has to be adjusted more or less frequently from every few hours to every few days depending on the stability of the temperature. The fibers were not adjusted during the measurement run.

For setting a particular state, polarizers are inserted after the long fibers in the measurement stations and coincidences between the transmitted photons are minimized by moving a half- and a quarter-wave plate (HWP, QWP) in the pump beam. For this state selection procedure, the photons were redirected by flip mirrors, placed in front of the electro-optic modulators (EOMs), to avalanche photo diodes (APDs). This way, all states of the form (S1) can be approximately obtained.

$$|\Psi\rangle = \frac{1}{\sqrt{1+r^2}} (|V\rangle_A |H\rangle_B + r |H\rangle_A |V\rangle_B) \quad (\text{S1})$$

To reduce the background, the SPDC photons are filtered spectrally with band-pass filters (BPF) with a FWHM of approximately 20 nm, and the crystal is placed in a heater at 162.5 °C. The rather high temperature has shown to reduce the background level of uncorrelated fluorescence. The crystal, 8 mm in length, with poling period 9.55  $\mu\text{m}$ , is slightly yawed with respect to the pump beam in order to reduce background counts from reflection at its surfaces.

Background counts seen by each detector when the laser is blocked have been estimated at less than one count per second.

## II. POLARIZATION MODULES

Each measurement station consists of a polarization module and a detector. It is necessary to select one of two linear polarizations, depending on the setting choice. For that, the light is coupled out of the fiber to pass a half-wave plate, an EOM, and a plate PBS [Fig. 1].

The transmitted output of the plate PBS is coupled into a fiber and transmitted to the TES for detection. The reflected output is recorded using an APD. This gives additional confirmation about the timing of photon arrivals (see Fig. 2) but is

\* marissa.giustina@univie.ac.at

† anton.zeilinger@univie.ac.at

otherwise neglected for the data analysis. Our EOM is a free space Pockels cell, consisting of two rubidium titanyl phosphate crystals. It is used as a fast polarization rotator so that the angles  $a_1$  and  $a_2$  for Alice ( $b_1$  and  $b_2$  for Bob) of the transmitted linear polarizations are  $32^\circ$  apart. The total transmission of the measurement module is approximately 92%. The Pockels cell is controlled by an FPGA board that reads random numbers from a random number generator [6, 7].

### III. RANDOM NUMBER GENERATORS

We use two accelerated laser phase diffusion random number generators (RNGs) of identical construction, designed and built at ICFO – The Institute of Photonic Sciences. The design, modeling, and testing of these devices is described in detail in [7]. As described there, each RNG continually generates partially random “raw” bits at a rate of 200 MHz and performs a running parity calculation to output processed bits that aggregate the randomness from all previous raw bits. At the time an output bit is taken for use as a measurement setting, only the most recent  $k$  raw bits will still be space-like separated from the distant measurement station, and thus only these  $k$  bits contribute local randomness. As described in the main text, the window for generation and processing of space-like separated raw bits is at least 26 ns, and thus  $k = 4$ . The predictability  $\mathcal{P}$  of the output (ideally  $\mathcal{P} = 1/2$  for a perfect random bit source) is  $\mathcal{P} \leq \frac{1}{2}(1 + \varepsilon_{\max}^{(k)})$ , where  $\varepsilon_{\max}^{(k)}$  bounds the excess predictability of the extracted bit. Due to the parity calculation,  $\varepsilon_{\max}^{(k)}$  decreases by roughly a factor of ten for each increment of  $k$ , reaching an experimentally useful bound of  $\varepsilon_{\max}^{(k)} \leq 2.4 \times 10^{-4}$  already for  $k = 4$ . The model uses a 6-sigma bound on untrusted noise sources and “fully paranoid” assumptions about how these noises combine [7], implying that setting choices with excess predictability larger than this occur with a frequency below  $2 \times 10^{-9}$ .

Alongside the model-based error bounds given above, high-volume statistical testing provides both support for the model-based calculations and a model-independent randomness check. Prior to the experiment the RNGs were tested at  $k = 4$ , achieved by keeping only every fourth output bit. As described in [7], we applied the test suites NIST SP800-22 [8] and more extensively TestU01 Alphabet battery [9], always finding results consistent with ideal randomness. The largest files tested contained  $2^{40}$  bits  $\approx 1$  Tb of data. The statistical uncertainty of a test of length  $2^{40}$  implies the ability to detect, with 1-sigma significance, correlations and other deviations from ideal randomness at the  $\frac{1}{\sqrt{2^{40}}}$  level. Producing such deviations requires at least predictability  $\mathcal{P} < \frac{1}{2}(1 + \frac{1}{\sqrt{2^{40}}}) = \frac{1}{2}(1 + 1.0 \times 10^{-6})$ . The  $k = 4$  output passes the tests at this level of precision, suggesting that the statistical metrology results are quite conservative.

The randomness harnessed in the RNGs originates in laser phase diffusion (LPD), a process driven by spontaneous emission. We note that the claimed randomness of the RNG is not restricted to quantum models. Both spontaneous emission and laser phase diffusion are observable and well-studied

processes, and any hypothesized classical or hidden-variable theory would also have to describe them. It is reasonable to expect that an important class of such models will describe spontaneous emission, and thus also LPD, as unpredictable, stochastic processes. Just as in quantum mechanics, for these non-quantum theories the phase is a good random variable, leading to unpredictable basis choices.

### IV. SPATIAL CONFIGURATION

We measured the spatial layout of our setup using a laser range finder and confirmed the results using a plan of the building. The distance between the emission event at the source and the closest edge of Alice’s RNG was measured to be  $29.23 \text{ m} \pm 0.04 \text{ m}$  while the distance between the emission event at the source and the closest edge of Bob’s RNG was measured to be  $28.96 \text{ m} \pm 0.04 \text{ m}$ . The actual production of the random bit takes place inside the RNG unit, thus these measurements conservatively quantify the distance between the emission and the random number generation. The measurements at Alice and Bob take place about 30 cm beyond the RNGs, so these measured values conservatively quantify the distance between the two stations. Deviations from a one-dimensional setup are sufficiently small to be negligible for the space-time configuration.

### V. DETECTORS

For photon detection, we employ fiber-coupled transition-edge sensors (TES). The TES is a calorimetric superconducting device cooled below its critical temperature ( $\sim 150 \text{ mK}$ ) but voltage biased to raise its electron temperature to within its superconducting transition, a region with steep temperature-resistance dependence. When heat is deposited by the absorption of a photon, the small change in temperature causes a measureable change in resistance. The corresponding change in current is measured by a low-noise SQUID current sensor [10, 11]. We operate both the TES and the SQUID in an adiabatic demagnetization refrigerator (ADR) at 100 mK.

To couple photons to the TES, we use an SMF-28 fiber with anti-reflection coating at 800 nm positioned over the detector. The TES are fabricated in an optical structure to optimize detection at 805 nm, thus we can expect detection efficiencies over 95% for these detectors [5, 12], including coupling from the SMF-28 fiber to the detector. The bare fiber passes into the ADR via a Teflon feed-through and is spliced to the SMF-28 fiber at the output port of the polarization module.

### VI. DATA RECORDING

The photon pair emission, random number generators, EOM switching, digitizers, and time-tagging modules at each measurement station are all synchronized to a “master clock” (function generator). To establish a common reference time

among all devices, a “zeroing” signal is distributed at the beginning of the experiment to all recording devices.

The chain of events involved in the measurement is as follows. The changing current signal in our TES from a single impinging 810 nm photon is on the order of 50 nA. This signal is amplified by a two-stage low-noise SQUID sensor (also at 100 mK) and room temperature amplifiers. The SQUID sensor is operated in a flux-locked loop. The comparably small TES current signal would not have required this. However, in our laboratory, a slowly changing magnetic field is present, for instance, from the Vienna Straßenbahn (tram), which runs almost directly above. Flux-locked loop operation linearizes the response of the SQUID sensor so that these magnetic background effects on the SQUID can be compensated by AC-coupling, thus ensuring stable operation. A further stage of room temperature amplification prepares the signal for recording by a 14-bit digitizer mounted in a PCI-Express bus of a computer where the data is written to hard disk. The amplified “photon” pulse has a height on the order of a few 100 mV with a rising edge of around 100 ns and a relaxation time of around 2  $\mu$ s. The digitizer operates in a triggered mode, recording in each trace 1 024 ns of pre-trigger and 1 024 ns of post-trigger data at a sample rate of 250 MHz whenever the signal crosses a threshold set aggressively to catch all photons and some noise (see Fig. S1). (The trigger level is set based on calibration data and takes a value in around 0.55 times the average photon height, depending on the signal to noise ratio of the SQUID-TES system.) After each trigger, the digitizer requires time to re-arm: up to 2 176 ns may pass before the next trigger can occur and in this time, the digitizer is blind. Each digitized trace has a timestamp, which enables accurate time-ordering of the collected data. The traces are evaluated for photons using a program that checks threshold crossings. All parameters of the algorithm are chosen using calibration data not part of any experimental runs. One threshold is responsible for the identification of a photon in a given trace, since the digitizer can also trigger on noise and record a trace that does not contain any photons. Thus a threshold fixed at a level around 0.75 times the average photon height (as found using calibration data) serves to determine the presence or absence of a photon. Another threshold fixed at a level around 0.2 times the average photon height assigns a timetag to the photon: the time when the identified photon’s signal crosses this threshold is recorded as the photon’s timetag. We assign a timestamp to each TES signal based on only local information and do not scan for coincidences anywhere in our experiment.

More detailed information on the detection scheme and space-time layout will be made available in [13].

## VII. DATA ANALYSIS

Before the experiment, we digitized and recorded over 250 000 traces per detector to use for calibrating the photon identification algorithms. We also recorded random settings at a rate of 1 MHz for about an hour in each RNG. Finally, we recorded experimental data for a total of approximately 4.8 hours. The first two blocks were predefined to be approxi-

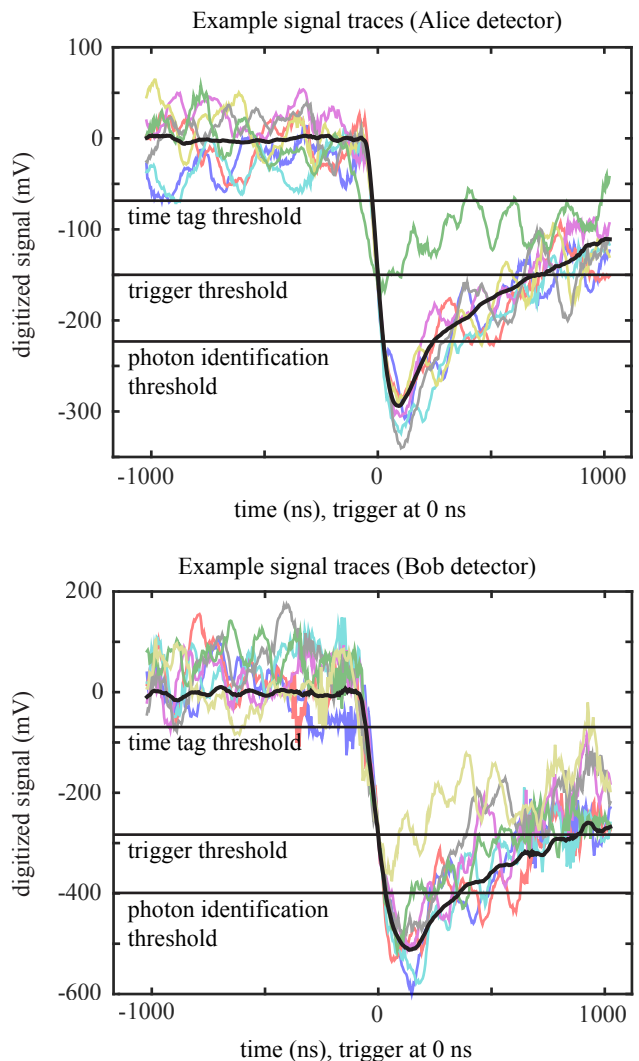

Figure S1. The solid black curves depict the photon signal shape in each detector, averaged from many traces containing identified photons. The colored curves show examples of individual traces recorded by the digitizer; not every recorded trace represents a photon at 810 nm (see for instance the green trace in the Alice detector and the yellow trace in the Bob detector). The three threshold levels are also depicted in these figures. The middle threshold is the level at which the digitizer triggers. Only signals that cross the lowest threshold can be identified as 810 nm photons. The time tag assigned to each photon is given by the time at which the signal crosses the upper time tag threshold.

mately one hour each; the remaining 2.8 hours were recorded in a single block. The recording was stopped when a real-time check monitoring the stability of the experiment (an estimate of the Bell value) indicated the setup was drifting out of alignment.

We choose rather arbitrarily to evaluate the second recorded block of data. It stems from 3 510 632 448 laser pulses (at rate 1 MHz) and thus possible pair emission events. However, after either digitizer triggers, it is not able to record data for the next two or three trials. These trials are flagged as invalid

and are not considered. This is justified because the decision that a trial will be invalid is reached using only data that was recorded before the setting choices or emission event for that trial have occurred. The number of valid trials is

$$N = 3\,502\,784\,150, \quad (\text{S2})$$

and the relevant counts are

$$N_{11} = 875\,683\,790, \quad N_{11}^{++} = 141\,439, \quad (\text{S3})$$

$$N_{12} = 875\,518\,074, \quad N_{12}^{+0} = 67\,941, \quad (\text{S4})$$

$$N_{21} = 875\,882\,007, \quad N_{21}^{0+} = 58\,742, \quad (\text{S5})$$

$$N_{22} = 875\,700\,279, \quad N_{22}^{++} = 8\,392. \quad (\text{S6})$$

Here  $N_{ij}$  is the number of trials with setting combination  $a_i b_j$ , and  $N_{ij}^{AB}$  is the number of trials in setting combination  $a_i b_j$  with outcome  $A \in \{+, 0\}$  for Alice and  $B \in \{+, 0\}$  for Bob. This gives the “Eberhard value” of counts

$$4(N_{11}^{++} - N_{12}^{+0} - N_{21}^{0+} - N_{22}^{++}) = 25\,456. \quad (\text{S7})$$

The factor of 4 is introduced here for consistency with the counting method below. A point estimate without any adjustments for the excess predictability gives the conditional probabilities  $p_{AB}(a_i b_j) = N_{ij}^{AB}/N_{ij}$ , and the  $J$ -value in the CH-Eberhard (CH-E) inequality becomes

$$\begin{aligned} J &\equiv p_{++}(a_1 b_1) - p_{+0}(a_1 b_2) - p_{0+}(a_2 b_1) - p_{++}(a_2 b_2) \\ &= 7.27 \times 10^{-6}, \end{aligned} \quad (\text{S8})$$

violating the local realist constraint  $J \leq 0$ .

To take into account the excess predictability of the RNGs, we follow the theoretical analysis in Ref. [14]. We assume that in every run the choices  $a$  and  $b$  of Alice and Bob are partially dependent on external influences that are in principle also available at the distant measurement events. We incorporate these influences, together with the hidden variable  $\lambda$  of the photon pair, into a joint hidden variable  $\mu$ . We assume that in every run,  $\mu$  influences the probability for a specific setting choice only to a certain extent, quantified by the parameters  $\varepsilon_A$  and  $\varepsilon_B$  for Alice and Bob respectively. As outlined in section III, these excess predictabilities (including bias) are  $\varepsilon_A = \varepsilon_B = 2.4 \times 10^{-4}$  with “6-sigma” certainty for each of them. Defining  $\varepsilon_{\pm} \equiv \varepsilon_A + \varepsilon_B \pm \varepsilon_A \varepsilon_B$ , this means that, in every trial, the probability to pick settings  $a$  and  $b$  (ideally  $\frac{1}{4}$ ) is assumed to obey

$$\frac{1}{4}(1 - \varepsilon_-) \leq p(a, b|\mu) \leq \frac{1}{4}(1 + \varepsilon_+). \quad (\text{S9})$$

The probability of “failure”—i.e.  $p(a, b|\mu)$  being outside one of the bounds—is less than  $q_f = 4 \times 10^{-9}$  (twice  $2 \times 10^{-9}$ , since the two RNGs can fail separately).

The small biases of the counts in Eqns. (S3–S6) are consistent with Eqn. (S9). The bound of Eqn. (S9) does allow partial dependence of the setting choices at Alice and Bob, and setting independence can be tested as discussed in [15]. However, Pearson’s  $\chi^2$ -test for independence,  $p(a_i b_j) = p(a_i)p(b_j)$ , does not indicate the presence of this effect. The test gives a probability of 0.787 that the observed data or

worse is obtained under the null hypothesis of independent setting choice (both with and without Yates’ continuity correction). Thus, based on the data in Eqns. (S3–S6), there is no evidence for dependent setting choice.

Nonetheless, we include the bound in Eqn. (S9) in an adapted CH-E inequality that takes excess predictability into account and reads [14]

$$\begin{aligned} J_{\varepsilon} &\equiv + \frac{p(++ , a_1 b_1)}{\frac{1}{4}(1 + \varepsilon_+)} - \frac{p(+0 , a_1 b_2)}{\frac{1}{4}(1 - \varepsilon_-)} \\ &\quad - \frac{p(0+ , a_2 b_1)}{\frac{1}{4}(1 - \varepsilon_-)} - \frac{p(++ , a_2 b_2)}{\frac{1}{4}(1 - \varepsilon_-)} \leq 0. \end{aligned} \quad (\text{S10})$$

The counting procedure works as follows: for every event  $X_{11}^{++}$ , i.e. when Alice chooses setting  $a_1$  and observes outcome  $+$  and Bob chooses  $b_1$  and observes outcome  $+$ , we add the increment  $\frac{4}{1+\varepsilon_+}$  to the process value  $Z_{J_{\varepsilon}}$ , and for each of the other three events  $X_{12}^{+0}, X_{21}^{0+}, X_{22}^{++}$  we add the (negative) increment  $\frac{-4}{1-\varepsilon_-}$  to the process value. By this procedure, including the factor of 4 in the increments, the expectation value for every increment is  $J_{\varepsilon}$  itself, making  $Z_{J_{\varepsilon}}$  a supermartingale. All other events are called “non-contributing”; these are mainly  $X_{ij}^{00}$  events without any photon registration but also events such as  $X_{12}^{++}$ , which do not contribute to the CH-E inequality either. After all  $N$  trials, we find the adapted CH-E process value

$$Z_{J_{\varepsilon}}^{(N)} = 24\,925.1. \quad (\text{S11})$$

This value is only slightly lower than the actual counts (S7). However, although the process value  $Z_{J_{\varepsilon}}^{(N)}$  is positive, the Hoeffding inequality does not give a useful bound on the  $p$ -value, which is the probability that local realism could have produced the data by a random variation. This is due to the large number of trials  $N$  and the fact that most of them are non-contributing. However, we can tighten the bound using Doob’s optional stopping theorem. There, we look at a “concentrated” version of the  $Z_{J_{\varepsilon}}$  process where we stop only at the contributing events ( $X_{11}^{++}, X_{12}^{+0}, X_{21}^{0+}, X_{22}^{++}$ ) and at the very last trial of the data set, whose length was chosen in advance. Therefore, the total number of (randomly distributed) “stopping times” and hence the length of the concentrated process is

$$M = N_{11}^{++} + N_{12}^{+0} + N_{21}^{0+} + N_{22}^{++} + 1 = 276\,515. \quad (\text{S12})$$

As we only omit events that do not contribute to the process value, the range of increments of the concentrated random process is still the maximum distance of the possible increments:

$$r_{J_{\varepsilon}} = \frac{4}{1+\varepsilon_+} + \frac{4}{1-\varepsilon_-} = 8.000\,001\,382. \quad (\text{S13})$$

The Hoeffding inequality then has the form

$$p(Z_{J_{\varepsilon}} \geq c\sqrt{M}) \leq e^{-\frac{2}{r_{J_{\varepsilon}}^2} c^2}. \quad (\text{S14})$$

For every number  $c$ , this expression bounds the probability that, after  $N$  trials, a local realist theory can obtain a process

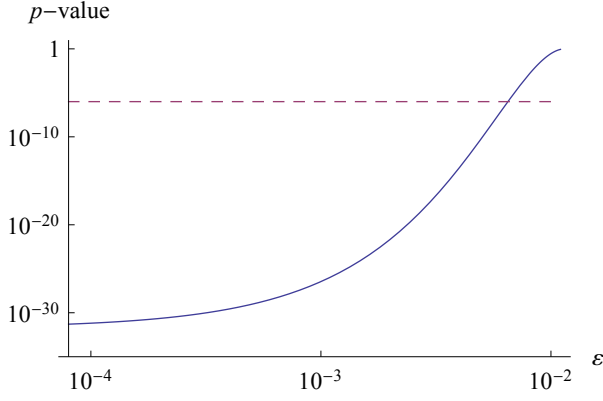

Figure S2. The solid line in this log-log graph shows the  $p$ -value as a function of the excess predictability  $\varepsilon$ . It remains below  $10^{-6}$  (dashed line) for excess predictability up to about 0.65 %.

value that is at least as large as  $c\sqrt{M}$ . Using  $c = Z_{J_\varepsilon}^{(N)} / \sqrt{M} = 47.40$ , this leads to a  $p$ -value of  $3.22 \times 10^{-31}$  for our data.

We also need to take possible failure of the bounds (S9) into account, where the adapted CH-E inequality (S10) does not apply. When it fails, the experimental trial in question could in principle saturate the algebraic bound, namely  $\frac{1}{1-\varepsilon_-}$ . To account for this, we subtract this algebraic upper bound times  $q_f$  in every trial, i.e. we add  $\frac{4}{1+\varepsilon_+} - \frac{q_f}{1-\varepsilon_-}$  for events  $X_{11}^{++}$ ,  $\frac{-1-q_f}{1-\varepsilon_-}$  for events  $X_{12}^{+0}$ ,  $X_{21}^{0+}$ ,  $X_{22}^{++}$ , and  $\frac{-q_f}{1-\varepsilon_-}$  for all the remaining (non-contributing) events. This adjusts the observed final process value to

$$Z_{K_\varepsilon}^{(N)} = Z_{J_\varepsilon}^{(N)} - N \frac{q_f}{1-\varepsilon_-} = 24\,911.1. \quad (\text{S15})$$

We now look again at a concentrated  $Z_{K_\varepsilon}$  process. As, in contrast to  $Z_{J_\varepsilon}$ , also the non-contributing trials contribute to the process  $Z_{K_\varepsilon}$ , its range—i.e. the range within which the increments from one stopping time to the next fall—changes. We choose to stop (in addition to the contributing events  $X_{11}^{++}$ ,  $X_{12}^{+0}$ ,  $X_{21}^{0+}$ ,  $X_{22}^{++}$ ), if there is a “streak” of more than  $s = 10^6$  non-contributing events in a row. This makes the range of the concentrated process

$$r_{K_\varepsilon} = r_{J_\varepsilon} + s \frac{q_f}{1-\varepsilon_-} = 8.004\,003\,303. \quad (\text{S16})$$

The longest streak in our data has length 165 190, so there are no additional stopping points because of this and we still have  $M$  stopping times. With these numbers, we find that

$$p(Z_{K_\varepsilon} \geq c\sqrt{M}) \leq e^{-\frac{2}{3} \frac{c^2}{r_{K_\varepsilon}^2}}. \quad (\text{S17})$$

Using  $c = Z_{K_\varepsilon}^{(N)} / \sqrt{M} = 47.37$ , we obtain a  $p$ -value of  $3.74 \times 10^{-31}$ . (We remark that it is also possible to keep the invalid trials and assign local ‘0’ outcomes within the detector recovery time. Then the  $p$ -value changes to  $3.97 \times 10^{-27}$ .)

We can speculate that there might be other adversarial influences on the setting choice that were not characterized in the experiment. We assume that the excess predictabilities for Alice’s and Bob’s settings are the same and label them with  $\varepsilon \equiv \varepsilon_A = \varepsilon_B$ . Fig. S2 shows a plot of the  $p$ -value as a function of  $\varepsilon$ , keeping a 6-sigma certainty for whatever the chosen number is. We can see that the  $p$ -value remains below the “gold standard” of  $10^{-6}$  up to the remarkably large excess predictability of about 0.65 %.

## VIII. NO-SIGNALING

We now check whether our data are in agreement with the principle of no-signaling. This principle demands that—under space-like separation—local outcome probabilities must not depend on the distant party’s setting. No-signaling must not only be obeyed in local realism but also in quantum mechanics, as its violation would contrast special relativity theory. Point estimates yield the following probabilities:

$$\begin{aligned} p_+^A(a_1 b_1) &= 2.45328 \times 10^{-4}, & p_+^A(a_1 b_2) &= 2.45308 \times 10^{-4}, \\ p_+^A(a_2 b_1) &= 6.66077 \times 10^{-4}, & p_+^A(a_2 b_2) &= 6.67851 \times 10^{-4}, \\ p_+^B(a_1 b_1) &= 2.48563 \times 10^{-4}, & p_+^B(a_2 b_1) &= 2.47842 \times 10^{-4}, \\ p_+^B(a_1 b_2) &= 5.40936 \times 10^{-4}, & p_+^B(a_2 b_2) &= 5.39428 \times 10^{-4}. \end{aligned} \quad (\text{S18})$$

Here,  $p_+^P(a_i b_j)$  is the probability that party P (A for Alice, B for Bob) observes outcome ‘+’ given setting choices  $a_i$  and  $b_j$ . Under the null hypothesis of no-signaling, the two conditional probabilities in each pair in (S18) should be equal. We perform a pooled two-proportion  $z$ -test to test for signaling, and the probabilities that the observed data or worse is obtained under the null hypothesis are 0.979, 0.151, 0.338, 0.174, respectively (avoiding Gaussian approximation would only give small differences to these probabilities). These large values do not require us to reject the null hypothesis of no-signaling.

- 
- [1] A. Fedrizzi, T. Herbst, A. Poppe, T. Jennewein, and A. Zeilinger, *Opt. Express*, **15**, 15377 (2007).  
 [2] M. Giustina, A. Mech, S. Ramelow, B. Wittmann, J. Kofler, J. Beyer, A. Lita, B. Calkins, T. Gerrits, S. W. Nam, R. Ursin, and A. Zeilinger, *Nature*, **497**, 227 (2013).

- [3] F. Steinlechner, *Sources of Photonic Entanglement for Applications in Space*, Ph.D. thesis, ICFO-Institut de Ciències Fòtoniques, Castelldefels, Barcelona, Spain (2015).  
 [4] R. S. Bennink, *Phys. Rev. A*, **81**, 053805 (2010).  
 [5] A. E. Lita, A. J. Miller, and S. W. Nam, *Opt. Express*, **16**, 3032 (2008).

- [6] C. Abellán, W. Amaya, M. Jofre, M. Curty, A. Acín, J. Capmany, V. Pruneri, and M. W. Mitchell, *Opt. Express*, **22**, 1645 (2014).
- [7] C. Abellán, W. Amaya, D. Mitrani, V. Pruneri, and M. W. Mitchell, *Phys. Rev. Lett.*, **115**, 250403 (2015).
- [8] A. Rukhin, J. Soto, J. Nechvatal, M. Smid, E. Barker, S. Leigh, M. Levenson, M. Vangel, D. Banks, A. Heckert, J. Dray, and S. Vo, *A Statistical Test Suite for Random and Pseudorandom Number Generators for Cryptographic Applications*, Tech. Rep. 800-22 (National Institute of Standards and Technology, 2010).
- [9] P. L'Ecuyer and R. Simard, *ACM Trans. Math. Softw.*, **33**, 22 (2007).
- [10] B. Cabrera, R. M. Clarke, P. Colling, A. J. Miller, S. W. Nam, and R. W. Romani, *Appl. Phys. Lett.*, **73**, 735 (1998).
- [11] D. Drung, C. Assmann, J. Beyer, A. Kirste, M. Peters, F. Ruede, and T. Schurig, *IEEE Trans. Appl. Supercond.*, **17**, 699 (2007).
- [12] A. E. Lita, B. Calkins, L. A. Pellouchoud, A. J. Miller, and S. W. Nam, in *Proc. SPIE 7681, Adv. Phot. Count. Tech. IV*, edited by M. A. Itzler and J. C. Campbell (2010).
- [13] M. Giustina, *In preparation*, Ph.D. thesis, University of Vienna, Vienna, Austria (2016).
- [14] J. Kofler, M. Giustina, J.-Å. Larsson, and M. W. Mitchell, (2015), arXiv:1411.4787.
- [15] A. Bednorz, (2015), arXiv:1511.03509.
